# Supplementary material for: Initial Guess Generation for Low-Thrust Trajectory Design with Robustness to Missed-Thrust-Events
Source: arXiv:2501.06694 source file (2025-01-12)
Supplement: Supplementary file 1 [file appendix.tex]

\section*{Appendix}
<INSERT>
